# Supplementary material for: The Fence Complexity of Persistent Sets
Source: arXiv:2309.05230 source file (2023-09-11)
Supplement: Supplementary file 2 [file appendix-background.tex]

\section{Detailed Overview of Related Techniques}

\myparagraph{Link and Persist}
The \LPList~technique is a general method for achieving durable linearizability in link-based data structures.
Using the \LPList~technique requires stealing one bit from every link in the data structure to use as a mark bit indicating whether or not the link has been written to persistent memory.
If the persistence bit is set then the link is not guaranteed have been written to persistent memory.
When a link is atomically updated the persistence bit is set.
The operation that set the bit must explicitly flush the link and perform a persistence fence then atomically remove the persistence mark.
Similarly, any operation that depends on the persistence of a link that has its persistence bit set must also explicitly flush the link and perform a persistence fence then atomically remove the persistence mark. 
 
\myparagraph{Link-Free}
The \LFList~algorithm achieved durable linearizability by adding two validity bits to every node. 
In their actual implementation the authors use byte sized fields to store the validity bits.
A node is considered in the data structure if both validity bits are set and the node is not marked as logically deleted. 
When a node is first allocated both bits are unset indicating that it is not valid. 
One of the validity bits is flipped when the node is in a transient state before it is actually inserted into the list. 
After inserting the other validity bit is set indicating that the node is in the list. 
Remove operations will only modify the validity bits when helping concurrent insert operations. 
The \LFList~ algorithm uses 2 separate flags to indicate when a psync was performed after inserting a node and after logically deleting a node. 
Read-only operations in the \LFList~ algorithm have upper bound psync complexity of 1. 

Compared to the \LPList~ technique, the \LFList~ algorithm reduces the number of required psyncs. 
However, not persisting the links of the data structure complicates the recovery procedure. 
The \LFList~ algorithm must completely rebuild the data structure during recovery. 
For this reason, it is clearly impossible for the \LFList~ algorithm to have an empty recovery procedure. 
Moreover, there is no way to quickly find all of the valid keys in persistent memory. 
This means that the recovery procedure for the \LFList~ algorithm must traverse every non-empty memory chunk held by the data structure to discover valid nodes.
Memory fragmentation becomes especially problematic for recovery. 
We can imagine a worst case scenario where every memory chunk contains only 1 valid node. 
The recovery procedure will still need to traverse the entire contents of every chunk. 
% For a large data structure this is especially problematic, a single threaded traversal and rebuilding would take a non-trivial amount of time.   

\myparagraph{SOFT}
Zuriel et al. \cite{zuriel2019efficient} designed a different algorithm called \SOFTList~ (Sets with an Optimal Flushing Technique) which meets the Cohen psync lower bound for update operations and requires no psyncs for read-only operations. 

Similar to their \LFList~ algorithm, the \SOFTList~ algorithm does not persist data structure links and instead persists metadata validity bits. 
One major difference between the \LFList~ algorithm and \SOFTList~ is that \SOFTList~ uses 2 different representations for every key in the data structure. 
Each key is stored in a volatile node which is never explicitly flushed to persistent memory and in a persistent which is explicitly flushed to persistent memory. 
The persistent node also contains the 3 metadata flags. 
The persistent nodes and volatile nodes are each allocated from separate dedicated regions of memory. 
Every volatile node contains a pointer to the corresponding persistent node. 
The pointer to the persistent node is also used to indicate the state of the node. 
A node can be in one of the 4 states: inserted, intent to insert, deleted or intent to delete. 
Inserts initially create a new volatile node with a corresponding persistent node which is in the state intend to insert. 
After a psync on persistent node the state is transitioned to inserted. Similarly, remove operations transition from intent to delete to deleted. 
A read-only operation can check the state of a persistent node to determine if the persistent node is durable which requires no psyncs. 

The \SOFTList~ algorithm reduces the number of required psyncs compared to the \LFList~ algorithm. 
The recovery procedure for \SOFTList~ is similar to that of the \LFList~ algorithm.
The recovery procedure must rebuild the entire data structure. 
To discover the keys that belong in the data structure, the recovery procedure must traverse every non-empty memory chunk that might contain persistent nodes.
