# Supplementary material for: The Fence Complexity of Persistent Sets
Source: arXiv:2309.05230 source file (2023-09-11)
Supplement: Supplementary file 5 [file appendix-evaluation.tex]

\section{Evaluation SWCAS vs DWCAS}
\label{section:swcas-vs-dwcas}

\begin{figure}[!t]
    \begin{subfigure}{0.24\textwidth}
        \centering
        \includegraphics[width=1\linewidth]{images/plots/clflush/throughput/swcas-vs-dwcas/Throughput-0.5_0.5-key=50.png}
        \caption{99\% Search, K = 50}
        \label{subfig:swcas-vs-dwcas-a}
    \end{subfigure}
    \begin{subfigure}{0.24\textwidth}
        \centering
        \includegraphics[width=1\linewidth]{images/plots/clflush/throughput/swcas-vs-dwcas/Throughput-25.0_25.0-key=50.png}
        \caption{50\% Search, K = 50}
        \label{subfig:swcas-vs-dwcas-b}
    \end{subfigure}
    \begin{subfigure}{0.24\textwidth}
        \centering
        \includegraphics[width=1\linewidth]{images/plots/clflush/throughput/swcas-vs-dwcas/Throughput-0.5_0.5-key=500.png}
        \caption{99\% Search, K = 500}
        \label{subfig:swcas-vs-dwcas-c}
    \end{subfigure}
    \begin{subfigure}{0.24\textwidth}
        \centering
        \includegraphics[width=1\linewidth]{images/plots/clflush/throughput/swcas-vs-dwcas/Throughput-25.0_25.0-key=500.png}
        \caption{50\% Search, K = 500}
        \label{subfig:swcas-vs-dwcas-d}
    \end{subfigure}
    \begin{subfigure}{1.0\textwidth}
        \centering
        \includegraphics[width=1\linewidth]{images/plots/clflush/throughput/swcas-vs-dwcas/legend.png}
    \end{subfigure}
    
    \caption{Persistent list throughput for our SWCAS implementations compared to DWCAS implementations. Y-axis represents operations per microsecond. X-axis represents the number of concurrent threads. K is the maximum key.}
    \label{fig:swcas-vs-dwcas}
\end{figure}

Figure \ref{fig:swcas-vs-dwcas} shows the throughput of our persistent list DWCAS versions compared to the SWCAS versions.
We find that, in practice, the DWCAS implementations of our list consistently out perform the SWCAS implementations.
For read-dominant workloads, the throughput achieved by the SWCAS implementations rivals that of the DWCAS implementations only when the size of the list is significantly larger than the number of threads.
In all other cases the DWCAS implementation achieves noticeably better throughput. 
This is likely due to the fact that the SWCAS requires significantly more volatile memory synchronization since the old pointer and next pointer of a node can be updated independently.
